# Supplementary material for: NumLLM: Numeric-Sensitive Large Language Model for Chinese Finance
Source: arXiv:2405.00566 source file (2024-05-01)
Supplement: Supplementary file 1 [file Appendix.tex]

\section{Experiments on Hyperparameters}

 There are three hyperparameters to study in the construction of NumLLM, including $n_{\text{min}}$, $r_{\text{ins}}$ and $r_{\text{NV}}$. $n_{\text{max}}$ changes according to  $n_{\text{min}}$ and is thus discussed together with $n_{\text{min}}$. We study the influence of each hyperparameter by training models with different values of that hyperparameter while holding the values of the remaining hyperparameters unchanged. The results are presented in Figure~\ref{figure:hpms}. 

Firstly, to study the influence of $n_{\text{min}}$ along with $n_{\text{max}}$, we train models with $n_{\text{min}}=1,3,10$, respectively. The corresponding value of $n_{\text{max}}$ is $2,8,20$, respectively. This group of hyperparameters influence the average length of each instruction. From Figure \ref{subfigure:n_min}, we can find that NumLLM achieves the best performance when $n_{\text{min}}=3$. The corresponding value of  $n_{\text{max}}$ is 8. One possible reason to explain this result is that, when  $n_{\text{min}}=1$, the average length of each instruction is too short and the context is not sufficient for the model to learn to predict the numeric variable. Meanwhile, when  $n_{\text{min}}=10$, the average length of each instruction is too  long and too many irrelevant texts are incorporated when learning the context dependency of the numeric variable. Both situations result in a drop in the model's performance.

Secondly, to study the influence of  $r_{\text{ins}}$, we train models with $r_{\text{ins}}=0.01,0.05,0.5,1$, respectively. $r_{\text{ins}}$ represents the randomness in numeric-sensitive instance extraction, which is meant to enhance the relevance of financial knowledge in the selected instances. From Figure \ref{subfigure:r_ins}, we can find that NumLLM achieves the best performance when $r_{\text{ins}}=0.05$. One possible reason to explain this result is that, when $r_{\text{ins}}=0.01$, too few instances are selected and the model cannot make full usage of the corpus. Meanwhile, when   $r_{\text{ins}}=0.5,1$, the occurrence of irrelevant texts in all the selected instances is too high, as discussed in section \ref{section:r_ins}. Both situations result in a drop in the model's performance.

Lastly, to study the influence of $r_{\text{NV}}$, we train models with $r_{\text{NV}}=0.1,0.3,0.8$, respectively.  $r_{\text{NV}}$ represents the randomness in numeric-masked choice generation, which is meant to maintain the diversity of instructions. From Figure \ref{subfigure:r_NV}, we can find that NumLLM achieves the best performance when $r_{\text{NV}}=0.3$. One possible reason to explain this result is that, when $r_{\text{NV}}=0.1$, too few numeric variables within the instance are selected and the model cannot make full exploitation of the corpus. Meanwhile, when   $r_{\text{NV}}=0.8$,most of the content of the instructions constructed from the same instance would be overlapped. This would impair diversity, as discussed in section \ref{section:r_NV}. Both situations result in a drop in the model's performance.
\begin{figure}[!t]
    \centering
    
\begin{subfigure}{0.55\linewidth}
    \centering
    \includegraphics[width=\linewidth]{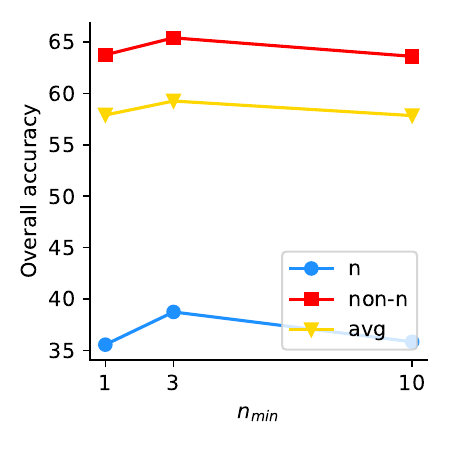}
    \caption{Influence of $n_{\text{min}}$}
    \label{subfigure:n_min}
\end{subfigure}
\begin{subfigure}{0.55\linewidth}
    \centering
    \includegraphics[width=\linewidth]{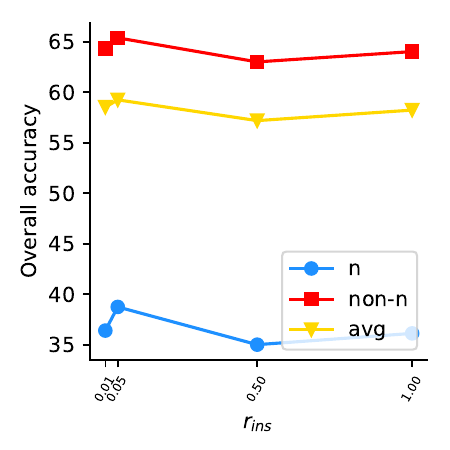}
    \caption{Influence of $r_{\text{ins}}$}
    \label{subfigure:r_ins}

\end{subfigure}
\begin{subfigure}{0.55\linewidth}
    \centering
    \includegraphics[width=\linewidth]{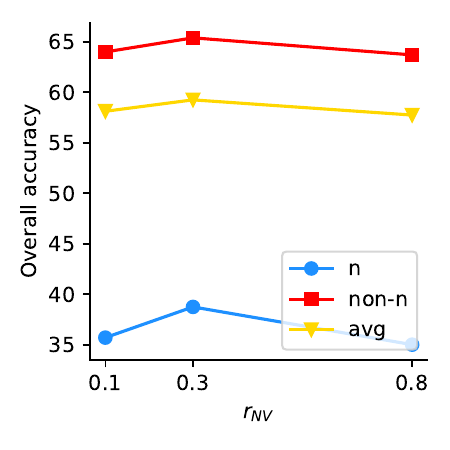}
    \caption{Influence of $r_{\text{NV}}$}
    \label{subfigure:r_NV}

\end{subfigure}

    \caption{Influence of hyperparameters, including $n_{\text{min}}$, $r_{\text{ins}}$ and $r_{\text{NV}}$.  ``n'' represents accuracy on numeric questions, ``non-n'' represents accuracy on non-numeric questions, and ``avg'' represents average accuracy over all the questions.}
    \label{figure:hpms}
\end{figure}

\begin{figure}[t]
    \centering
    
\begin{subfigure}{\linewidth}
    \centering
    \includegraphics[width=\linewidth]{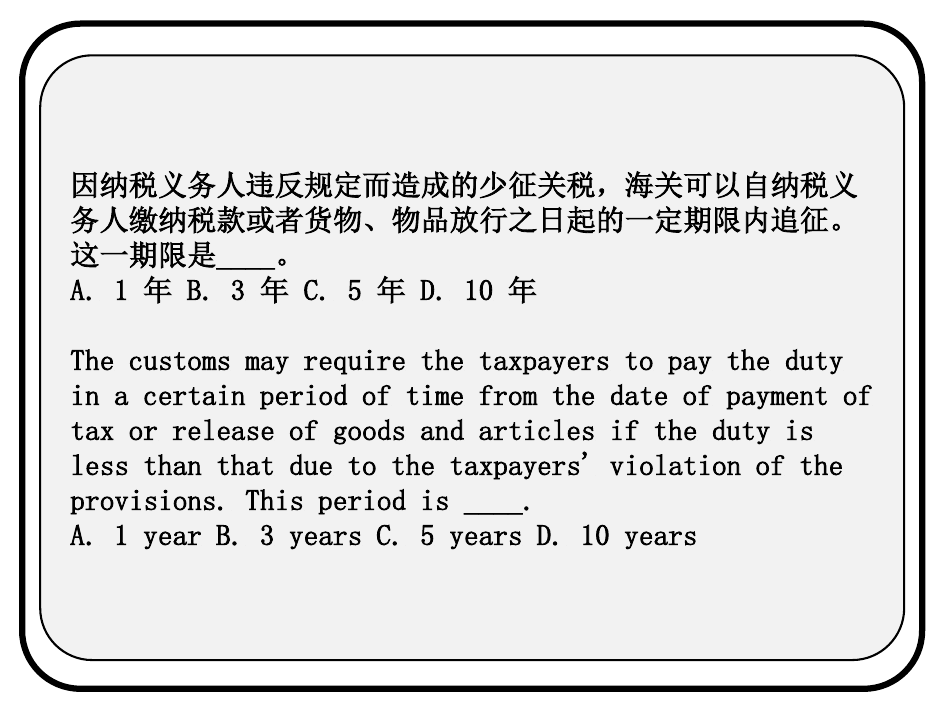}
\end{subfigure}
\begin{subfigure}{\linewidth}
    \centering
    \includegraphics[width=\linewidth]{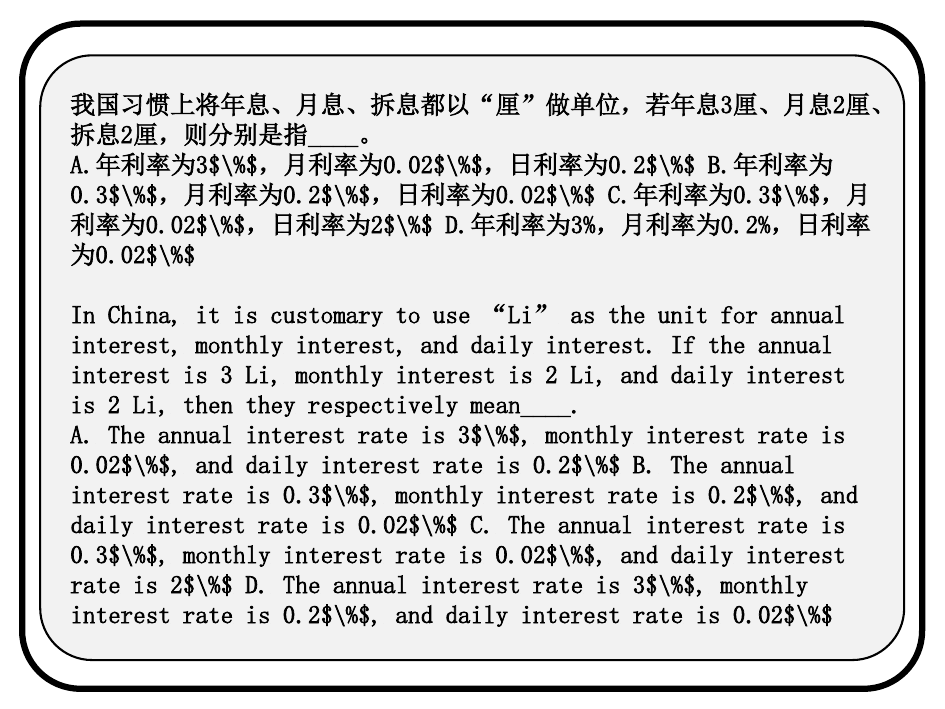}
\end{subfigure}
\begin{subfigure}{\linewidth}
    \centering
    \includegraphics[width=\linewidth]{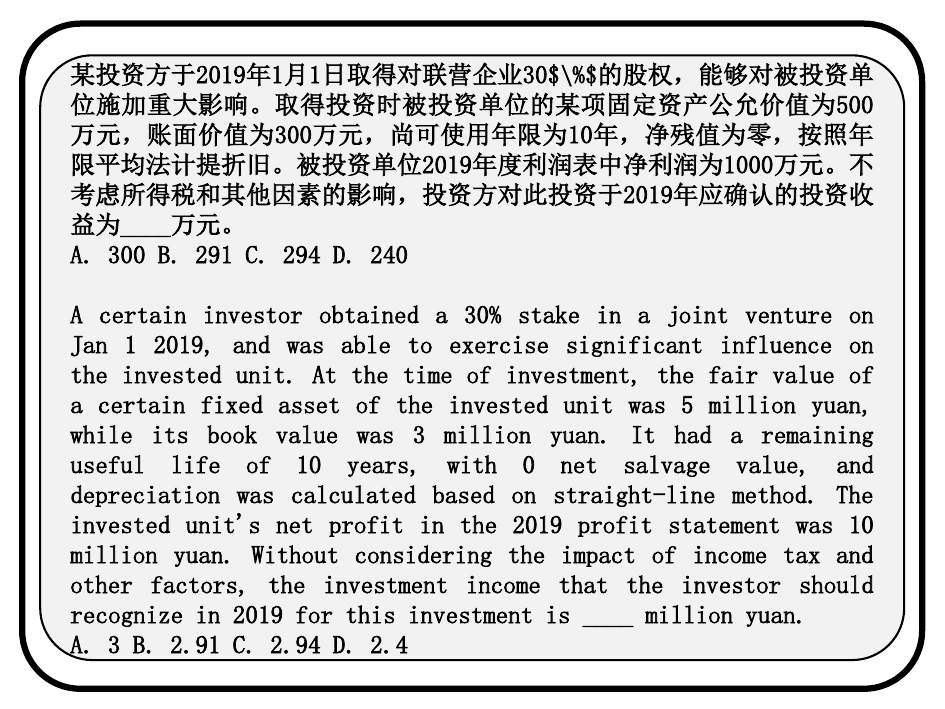}
\end{subfigure}

    \caption{Examples of numeric questions}
    \label{figure:numeric}
\end{figure}

\begin{figure}[t]
    \centering
    
\begin{subfigure}{\linewidth}
    \centering
    \includegraphics[width=\linewidth]{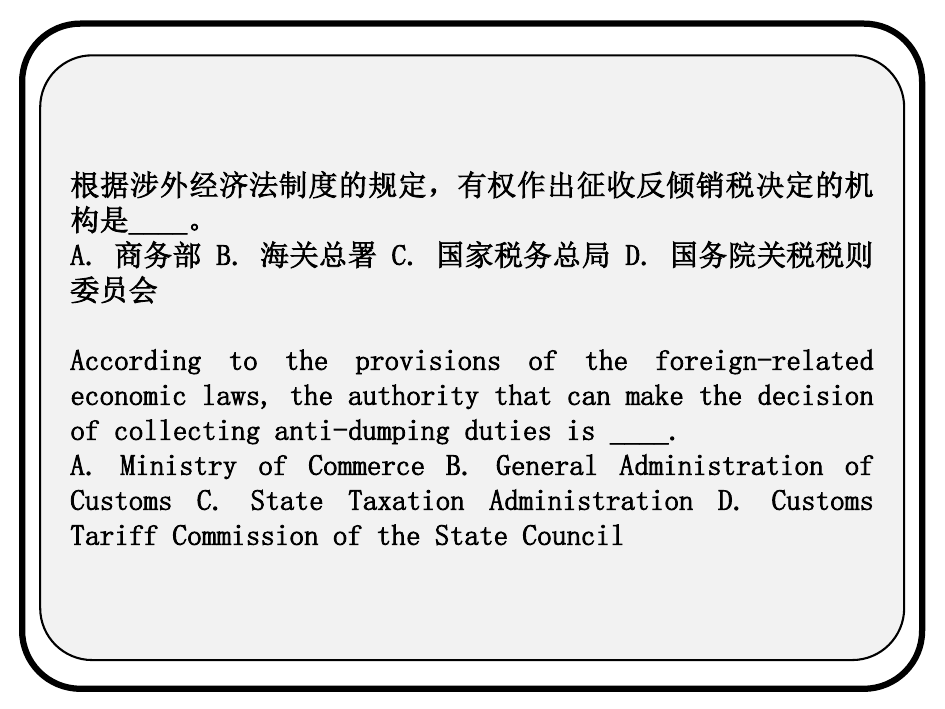}
\end{subfigure}
\begin{subfigure}{\linewidth}
    \centering
    \includegraphics[width=\linewidth]{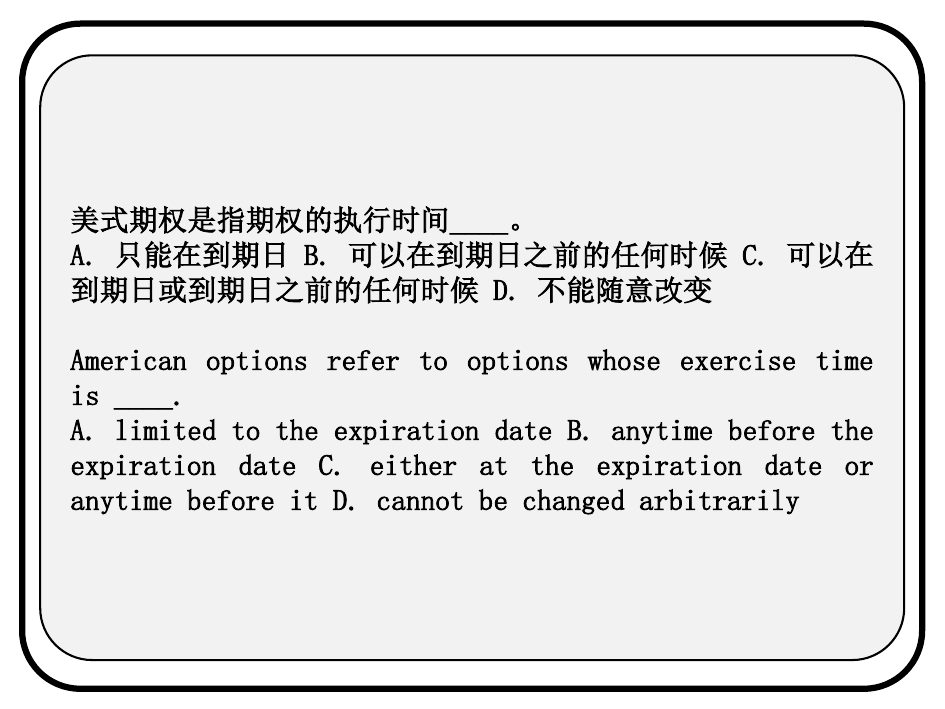}

\end{subfigure}
\begin{subfigure}{\linewidth}
    \centering
    \includegraphics[width=\linewidth]{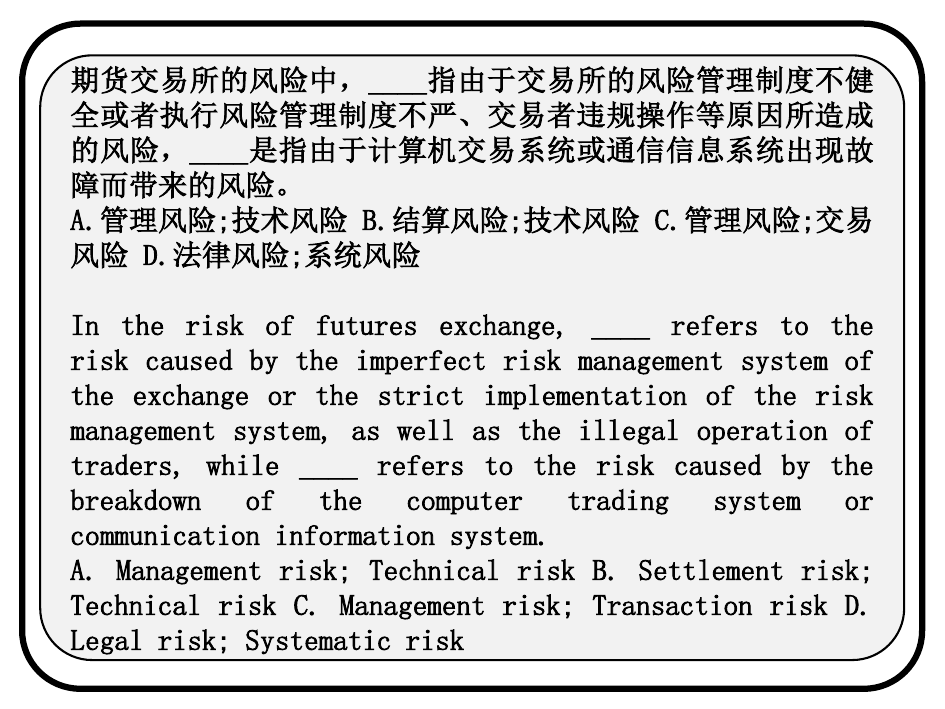}

\end{subfigure}
    \caption{Examples of non-numeric questions}
    \label{figure:non-numeric}
\end{figure}
\section{More Examples of Numeric and Non-Numeric Questions}

As discussed in section \ref{section:Evaluation Tasks}, we decompose all questions within each sub-domain in the benchmark into numeric questions and non-numeric questions. We define numeric questions as those whose options contain numeric variables, in contrast to non-numeric questions. More examples of numeric questions are listed in Figure \ref{figure:numeric}, and more non-numeric questions are listed in Figure \ref{figure:non-numeric}.
